# Supplementary material for: LoRC: Low-Rank Compression for LLMs KV Cache with a Progressive Compression Strategy
Source: arXiv:2410.03111 source file (2024-10-04)
Supplement: Supplementary file 1 [file appendix_prompts.tex]

\section{Prompts used in experiments}
We present our prompts used for different datasets here. We use a few-shot setting for LLaMA-2 models on OpenBookQA (1-shot), BoolQ (2-shot), and GSM8k (8-shot), and zero-shot setting for other experiments.

\textbf{OpenBookQA}
\begin{lstlisting}[language=Python]
def format_examples(examples):
    example_prompts = []
    for j in range(1):
        question = examples['question_stem'][j]
        fact = examples['fact1'][j]
        choices = examples['choices'][j]['text']
        labels = examples['choices'][j]['label']
        formatted_choices = "\n".join(f"{label}) {text}" for label, text in zip(labels, choices))
        answer = examples['answerKey'][j]
        example_prompt = f"Fact: {fact}\nQuestion: {question}\nOptions:\n{formatted_choices}\nAnswer: {answer}\n"
        example_prompts.append(example_prompt)
    return "\n---\n".join(example_prompts)


def create_prompts_from_data(data, example_context):
    prompts = []
    answers = []
    for i in range(len(data['id'])):
        question = data['question_stem'][i]
        fact = data['fact1'][i]
        choices = data['choices'][i]['text']
        labels = data['choices'][i]['label']
        formatted_choices = "\n".join(f"{label}) {text}" for label, text in zip(labels, choices))

        task_intro = "You will be provided with a fact and a related question. Your task is to use the given fact to choose the correct answer from the provided options."
        prompt = f"Task Introduction:\n{task_intro}\n1-Shot Examples:\n{example_context}\n---\nFact: {fact}\nQuestion: {question}\nOptions:\n{formatted_choices}\nAnswer:"
        prompts.append(prompt)
        answers.append(data['answerKey'][i])
    return prompts, answers


def extract_option_label(outputs):
    answer_labels = []
    for output in outputs:
        match = re.search(r'\b([A-D])\b', output)
        if match:
            answer_labels.append(match.group(1))
        else:
            answer_labels.append(None)
    return answer_labels
\end{lstlisting}

\textbf{BoolQ}
\begin{lstlisting}[language=Python]
def get_examples(dataset, num_examples):
    selected_examples = dataset.shuffle(seed=42).select(range(num_examples))
    examples = []
    for i in range(num_examples):
        passage = selected_examples['passage'][i]
        question = selected_examples['question'][i]
        answer = "yes" if selected_examples['answer'][i] else "no"
        examples.append((passage, question, answer))

    example_section = "\n\n".join([
        f"Example {i + 1}:\nPassage: {ex[0]}\nQuestion: {ex[1]}\nAnswer: {ex[2]}" for i, ex in enumerate(examples)
    ])
    return example_section

def create_prompts_from_data(data, example_section=None):
    task_description = "For each passage and question, determine if the answer to the question is 'yes' or 'no' based on the passage provided."

    prompts = []
    references = []
    for question, passage, answer in zip(data['question'], data['passage'], data['answer']):
        prompt = f"{task_description}\n\n2-Shot Examples:{example_section}\n\nPassage: {passage}\nQuestion: {question}\n\nAnswer (yes or no):"
        prompts.append(prompt)
        references.append("yes" if answer else "no")
    return prompts, references

def extract_answer(generated_text: str) -> str:
    normalized_text = generated_text.lower().strip()
    if normalized_text.startswith("yes"):
        return "yes"
    elif normalized_text.startswith("no"):
        return "no"
    return "unknown"
\end{lstlisting}

\textbf{XSum}
\begin{lstlisting}[language=Python]
def create_prompts_from_data(data):
    prompts = []
    references = []
    for article, summary in zip(data['document'], data['summary']):
        prompt = f"Provide a concise summary of the text below: {article}\n\nSummary:"
        prompts.append(prompt)
        references.append(summary)
    return prompts, references
\end{lstlisting}

\textbf{GSM8k}
\begin{lstlisting}[language=Python]
def create_prompts_from_data(data, examples):
    content = f"Please give a step-by-step answer to the question. You have to put your final numeric answer at the end, without any extra sign, prefix, or suffix, just pure integer numbers, in the format: \n#### answer\n Done, make sure to separate the final numeric answer with \n####"

    prompts = []
    references = []

    example_section = ""
    for ex_question, ex_answer in examples:
        example_section += f"\nExample Question: {ex_question}\nExample Answer: {ex_answer}\n"

    for question, answer in zip(data['question'], data['answer']):
        prompt = f"{example_section}\nQuestion: {question}\n{content}."
        prompts.append(prompt)
        _, extracted_answer = extract_answer(answer)
        references.append(extracted_answer)
    return prompts, references

def extract_answer(completion):
    start_idx = completion.find("####")
    if start_idx == -1:
        return completion, 'None'
    start_idx += 4  # Move past '####'
    end_idx = completion.find('\n', start_idx)
    if end_idx == -1:
        end_idx = len(completion)
    answer = completion[start_idx:end_idx].strip()
    return completion[:end_idx], answer


def calculate_accuracy(predictions, references):
    correct = sum([1 for (_, pred), ref in zip(predictions, references) if pred.lower() == ref.lower()])
    return correct, len(predictions)
\end{lstlisting}
